# Supplementary material for: Smooth, exact rotational symmetrization for deep learning on point clouds
Source: arXiv:2305.19302 source file (2024-02-06)
Supplement: Supplementary file 1 [file SI.pdf]

# 1 Counterexample explanation

The paper[] suggests a general recipe to construct universal approximators on point clouds. The specific example is given for a point cloud consisting of 5 points additionally supplied with a scalar property which authors name a mass. The goal is to learn a rotationally covariant and permutationally invariant function $h$:

$$h \,:\, (\mathbb{R} \times \mathbb{R}^3) \to \mathbb{R}^{3\times 3} \tag{1}$$

The function $h$ associates rotationally covariant matrix to the point cloud and this mapping is invariant with respect to the permutation of the points in the point cloud.

It is falsely claimed that any such function $h$ can be represented in the form:

$$h((m_i, x_i)_{i=1}^5) = \sum_{i=1}^{5} f_0(x_i^T x_i, m_i, \{x_k^T x_l, m_k, m_l\}_{k,l\neq i}) x_i x_j^T + \\ \sum_{i>j=1}^{5} f_1(x_i^T x_j, m_i, m_j, \{x_k^T x_l, m_k, m_l\}_{k,l\neq i,j}) x_i x_j^T + f_2(\{x_i^T x_j, m_i, m_j\}_{i,j=1}^5) I \tag{2}$$

where $I$ means identity matrix and {...} expressions mean unordered sets.

We show that this claim is wrong by providing an explicit counterexample showing such a function $h$ and such point clouds that the value of $h$ on these point clouds can not be represented in the form of Eq. **??**

In our counterexample all the masses are equal to each other, thus, it is possible to simplify expression **??** to:

$$h((x_i)_{i=1}^5) = \sum_{i=1}^{5} f_0(x_i^T x_i, \{x_k^T x_l, \}_{k,l\neq i}) x_i x_j^T + \sum_{i>j=1}^{5} f_1(x_i^T x_j, \{x_k^T x_l\}_{k,l\neq i,j}) x_i x_j^T \\ + f_2(\{x_i^T x_j\}_{i,j=1}^5) I \tag{3}$$

The coordinates of the first set of points is given by:

$$(x_i^{first})_{i=1}^5 = \begin{bmatrix} 1 & -1 & 2 & -2 & 0 \\ 1 & -1 & 0 & 0 & 1 \\ 0 & 0 & 2 & -2 & 1 \end{bmatrix} \tag{4}$$

The coordinates of second:

$$(x_i^{second})_{i=1}^5 = \begin{bmatrix} 1 & -1 & 2 & -2 & 0 \\ 1 & -1 & 0 & 0 & 1 \\ 0 & 0 & 2 & -2 & -1 \end{bmatrix} \tag{5}$$

The function $h$ is given by:

$$h((x_i)_{i=1}^5) = \sum_i \lambda_i^3 I \tag{6}$$

Where $\lambda_i$ are eigenvalues of the corresponding Gram matrix.

It is clear that this expression is rotationally covariant and invariant with respect to permutation of the points in the point cloud. The value of the function $h$ for the first point cloud is:

$$h((x_i^{first})_{i=1}^5) = \begin{bmatrix} 5692 & 0 & \\ 0 & 5692 & 0 \\ 0 & 0 & 5692 \end{bmatrix} \tag{7}$$

;

The value for the second is:

$$h((x_i^{second})_{i=1}^5) = \begin{bmatrix} 5500 & 0 & \\ 0 & 5500 & 0 \\ 0 & 0 & 5500 \end{bmatrix} \tag{8}$$

We analyze the difference of the two predictions given by representation **??**:

$$h((x_i^{first})_{i=1}^5) - h((x_i^{second})_{i=1}^5) = Delta_0 + Delta_1 + Delta_2 \tag{9}$$

, where

$$Delta_0 = \sum_{i=1}^5 f_0((x_i^{first})^T x_i^{first}, \{(x_k^{first})^T x_l^{first}, \}_{k,l \neq i}) x_i^{first} (x_j^{first})^T - \sum_{i=1}^5 f_0((x_i^{second})^T x_i^{second}, \{(x_k^{second})^T x_l^{second}, \}_{k,l \neq i}) x_i^{second} (x_j^{second})^T \tag{10}$$

$$Delta_1 = \sum_{i>j=1}^5 f_1((x_i^{first})^T x_j^{first}, \{(x_k^{first})^T x_l^{first}\}_{k,l \neq i,j}) x_i^{first} (x_j^{first})^T - \sum_{i>j=1}^5 f_1((x_i^{second})^T x_j^{second}, \{(x_k^{second})^T x_l^{second}\}_{k,l \neq i,j}) x_i^{second} (x_j^{second})^T \tag{11}$$

$$Delta_2 = f_2(\{(x_i^{first})^T x_j^{first}\}_{i,j=1}^5) I - f_2(\{(x_i^{second})^T x_j^{second}\}_{i,j=1}^5) I \tag{12}$$

The expression **??** contains 10 terms in total, but out of these terms only 5 arguments to the function $f_0$ are unique. These unique arguments are:

$$\zeta_1 = (2, \{-8, -8, -2, -2, -2, -2, -1, -1, 2, 2, 2, 2, 2, 2, 8, 8\})$$
$$\zeta_2 = (2, \{-8, -8, -2, -2, -2, -2, 1, 1, 2, 2, 2, 2, 2, 2, 8, 8\})$$
$$\zeta_3 = (8, \{-2, -2, -2, -2, -2, -2, -1, -1, 1, 1, 2, 2, 2, 2, 2, 8\})$$
$$\zeta_4 = (8, \{-2, -2, -2, -2, -1, -1, 1, 1, 2, 2, 2, 2, 2, 2, 8\})$$
$$\zeta_5 = (2, \{-8, -8, -2, -2, -2, -2, -2, -2, 2, 2, 2, 2, 2, 2, 8, 8\})$$

, which implies that $Delta_0$ can be written in the form:

$$Delta_0 = f_0(2, \{-8, -8, -2, -2, -2, -2, -2, -2, 2, 2, 2, 2, 2, 2, 8, 8\}) \begin{bmatrix} 0 & 0 & 0 \\ 0 & 0 & 2 \\ 0 & 2 & 0 \end{bmatrix} = \begin{bmatrix} 0 & 0 & 0 \\ 0 & 0 & 2f_0(\zeta_5) \\ 0 & 2f_0(\zeta_5) & 0 \end{bmatrix} \quad (13)$$

.

Similarly the expression for $Delta_1$ contains 20 terms, but out of these 20 there are only 5 unique arguments to the function $f_1$. These arguments are:

$$\kappa_1 = (-2, \{-8, -8, -2, -2, -2, -2, -2, -2, -2, -1, -1, 1, 1, 2, 2, 2, 2, 2, 2, 2, 2, 2, 8, 8\})$$
$$\kappa_2 = (2, \{-8, -8, -2, -2, -2, -2, -2, -2, -2, -2, -1, -1, 1, 1, 2, 2, 2, 2, 2, 2, 2, 2, 8, 8\})$$
$$\kappa_3 = (1, \{-8, -8, -2, -2, -2, -2, -2, -2, -2, -2, -1, -1, 1, 2, 2, 2, 2, 2, 2, 2, 2, 2, 8, 8\})$$
$$\kappa_4 = (-1, \{-8, -8, -2, -2, -2, -2, -2, -2, -2, -2, -1, 1, 1, 2, 2, 2, 2, 2, 2, 2, 2, 2, 8, 8\})$$
$$\kappa_5 = (-8, \{-8, -2, -2, -2, -2, -2, -2, -2, -2, -1, -1, 1, 1, 2, 2, 2, 2, 2, 2, 2, 2, 2, 8, 8\})$$

Which implies that $Delta_1$ can be written in the form:

$$Delta_1 = \begin{bmatrix} 0 & -4f_1(\kappa_1) + 4f_1(\kappa_2) & 2f_1(\kappa_3) - 2f_1(\kappa_4) \\ 0 & 0 & 2f_1(\kappa_3) - 2f_1(\kappa_4) \\ 0 & -4f_1(\kappa_1) + 4f_1(\kappa_2) & 0 \end{bmatrix} \quad (14)$$

Since the unordered sets of the elements of Gram matrices for these two point clouds are exactly identical (given by

$$\{-8, -8, -2, -2, -2, -2, -2, -2, -2, -2, -1, -1, 1, 1, 2, 2, 2, 2, 2, 2, 2, 2, 2, 2, 8, 8\}$$

(15)

) the $Delta_2 = 0$.

Assembling all this analysis together we obtain that

$$h((x_i^{first})_{i=1}^5) - h((x_i^{second})_{i=1}^5) =$$
$$\begin{bmatrix} 0 & -4f_1(\kappa_1) + 4f_1(\kappa_2) & 2f_1(\kappa_3) - 2f_1(\kappa_4) \\ 0 & 0 & 2f_1(\kappa_3) - 2f_1(\kappa_4) + 2f_0(\zeta_5) \\ 0 & -4f_1(\kappa_1) + 4f_1(\kappa_2) + 2f_0(\zeta_5) & 0 \end{bmatrix} = \tag{16}$$
$$\begin{bmatrix} 192 & 0 & \\ 0 & 192 & 0 \\ 0 & 0 & 192 \end{bmatrix}$$

Apparently, this equality can not be satisfied with any functions $f_0$, $f_1$ and $f_2$ since $192 \neq 0$ which implies that the statement from [] that any rotationally covariant and permutationally invariant function $h$ can be represented in the form of **??** is wrong. This, in turn, implies that a recipe to construct of universal approximators is wrong and constructed functional forms are not able to fit certain ground truth functional dependencies.

*****************OUTDATED BELOW *********************

Thus, the corresponding gram matrices are:

$$G_1 = \begin{bmatrix} 2 & -2 & 2 & -2 & 1 \\ -2 & 2 & -2 & 2 & -1 \\ 2 & -2 & 8 & -8 & 2 \\ -2 & 2 & -8 & 8 & -2 \\ 1 & -1 & 2 & -2 & 2 \end{bmatrix} \tag{17}$$

and

$$G_2 = \begin{bmatrix} 2 & -2 & 2 & -2 & 1 \\ -2 & 2 & -2 & 2 & -1 \\ 2 & -2 & 8 & -8 & -2 \\ -2 & 2 & -8 & 8 & 2 \\ 1 & -1 & -2 & 2 & 2 \end{bmatrix} \tag{18}$$

The sets of eigenvalues for these gram matrices are not the same, which means that point clouds can not be superposed by rigid transformations:

$$\{\lambda_1\} = \{0.000, 0.000, 1.212, 2.962, 17.826\} \tag{19}$$

$$\{\lambda_2\} = \{0.000, 0.000, 0.000, 4.443, 17.557\} \tag{20}$$
