# Supplementary material for: Smooth, exact rotational symmetrization for deep learning on point clouds
Source: arXiv:2305.19302 source file (2024-02-06)
Supplement: Supplementary file 3 [file si-body-old.tex]

\section{sp made computationally efficient}


* additional cutting for each pair [2, 4] $\rightarrow$ [1, 2] depending on presence or absence of inversional invariance

First of all, one can notice that the weights associated with the reference given in eq. \ref{eq:weight_full} are symmetric $w_{ij} = w{ji}$. It means that the expression \ref{eq:weighted_average} can be rewritten as:
\begin{equation}
SP(\chi) = \frac{\sum\limits_{i < j} w_{ij} [D_{Y}[g_{ij}] 
 IM(D_{X} [g^{-1}_{ij}]\chi) + D_{Y}[g_{ji}] 
 IM(D_{X} [g^{-1}_{ji}]\chi) ] }{\sum\limits_{ij} w_{ij}}
\end{equation}

\begin{figure}[tb]
    \centering
    \includegraphics[width=0.8\linewidth]{figures/filtering_ordered_pairs.jpg}
    \caption{filtering ordered pairs}
    \label{fig:filtering_ordered_pairs}
\end{figure}



\begin{widetext}
\begin{equation}
\begin{split}
&D_{Y}[g_{ij}] 
 IM(D_{X} [g^{-1}_{ij}]\chi) + D_{Y}[g_{ji}] 
 IM(D_{X} [g^{-1}_{ji}]\chi)  \to \\
&\to \frac{D_{Y}[g_{ij}] 
 IM(D_{X} [g^{-1}_{ij}]\chi)q(r_1 - r_2 | -\Delta, C_r) + D_{Y}[g_{ji}] 
 IM(D_{X} [g^{-1}_{ji}]\chi) q (-(r_1 - r_2) | \Delta, C_r)}{q(r_1 - r_2 | -\Delta, C_r) + q (-(r_1 - r_2) | \Delta, C_r)}
\end{split}
\end{equation}
\end{widetext}
It is illustrated in the Fig. \ref{fig:symmetrization_protocol} I. Thus, most of the time only one reference frame is associated to an unordered pair of neighbors - the one, where the first neighbor is the furthest one. In a narrow transition region determined by $\Delta$ two reference frames are used with smooth stitching.

\onecolumngrid
\section{Full pipeline for the first all-collinear solution}
\mycomment{Discuss smth for the case when SP is applied for center of the mass, and thus, some point can coincide with each other}. 

\begin{algorithm}
\hspace*{\algorithmicindent} \textbf{Constant parameters: } $\gamma > 0; \beta > 0; C > 0; \Delta_r > 0$. 

\hspace*{\algorithmicindent} \textbf{Parameter units: } The units of  $\Delta_r$ is length; the units of $\beta$ is inverse length,  all the other parameters are dimensionless\\
\begin{algorithmic}[1]
\STATE Estimate/take as a reasonable constant $R_{cut}^{outer} > R_{cut}^{IM}$
\STATE $R_{cut}^{outer} \gets R_{cut}^{outer}(1 + \gamma)$
\FOR {$i, j: r_i, r_j \leq R_{cut}^{outer}$}
  \STATE $psm_{ij} \gets \text{SmoothMax}_{\beta}(\{r_i, r_j\}) + T(\beta)$
  \STATE $p_{ij} \gets f_c(r_i | R_{cut}^{outer}, C) f_c(r_j | R_{cut}^{outer}, C) q(\lVert \hat{r_i} \times \hat{r_j}\rVert_2^2 | \Delta, C)$
\ENDFOR
\STATE $R_{cut}^{inner} \gets {\text{SmoothMinWeighted}_{\beta}}(\{(psm_{ij}, p_{ij})| i, j: r_i, r_j \leq R_{cut}^{outer}\} \cup \{(R_{cut}, 1.0)\})$
\FOR {$i, j: r_i, r_j \leq R_{cut}^{inner}$}
\STATE $\Delta_{ij} \gets {\lVert \hat{r_i} \times \hat{r_j} \rVert}_2^2$
\STATE $p\Delta_{ij} \gets  f_c(r_i| R_{cut}^{inner}, C) f_c(r_j | R_{cut}^{inner}, C) $
\ENDFOR
\STATE $\Delta_{adaptive} \gets {\text{SmoothMaxWeighted}_{\beta}}(\{(\Delta_{ij}, p\Delta_{ij})| i, j: r_i, r_j \leq R_{cut}^{inner}\})$

\STATE $R_{cut}^{inner} \gets R_{cut}^{inner} (1 + \gamma)$

\FOR {$i, j: r_i, r_j \leq R_{cut}^{inner} $ \textbf{ and } $i < j$}
\STATE $w_{ij} \gets fc(r_i | R_{cut}, C) fc(r_j | R_{cut}, C) q({\lVert \hat{r_i} \times \hat{r_j} \rVert}_2^2 | \Delta_{adaptive}, C)$
\IF {$w_{ij} > 0$}
\SWITCH{$r_i - r_j$}
    \CASE{$r_i - r_j \geq \Delta_r$}
      \STATE $\text{Prediction}_{ij} \gets D_{Y}[g_{ij}] 
 IM(D_{X} [g^{-1}_{ij}]\chi)$
    \ENDCASE
    \CASE{$-\Delta_r \leq r_i - r_j  \leq \Delta_r$}
      \STATE $\text{Prediction}_{ij} \gets \frac{D_{Y}[g_{ij}] 
 IM(D_{X} [g^{-1}_{ij}]\chi) q(r_i - r_j | -\Delta_r, C) + D_{Y}[g_{ji}] 
 IM(D_{X} [g^{-1}_{ji}]\chi) q (-(r_j - r_i) | \Delta_r, C)}{q(r_i - r_j | -\Delta_r, C) + q (-(r_j - r_i) | \Delta_r, C)}$
    \ENDCASE
    \CASE{$r_i - r_j \leq -\Delta_r$}
      \STATE $\text{Prediction}_{ij} \gets D_{Y}[g_{ji}] 
 IM(D_{X} [g^{-1}_{ji}]\chi)$ 
    \ENDCASE
\ENDSWITCH
\ENDIF
\ENDFOR


\STATE $\text{Prediction} \gets  \frac{\sum\limits_{i > j: r_i, r_j \leq R_{cut}^{inner}} w_{ij} Prediction_{ij}}{\sum\limits_{i > j: r_i, r_j \leq R_{cut}^{inner}} w_{ij} }$

\end{algorithmic}
\end{algorithm}
\subsection{Full pipeline for the second all-collinear solution}

\begin{equation}
{\text{SmoothMinWeighted}_{\beta}}(\{(psm_{ij}, p_{ij}) | i, j: r_i, r_j \leq R_{cut}^{outer}\} \cup \{(R_{cut}, 1.0)\})
\end{equation}

\begin{algorithm}
\hspace*{\algorithmicindent} \textbf{Constant parameters: } $\gamma > 0; \beta > 0; C > 0; 0 < \Delta < 1; \Delta < \Delta_{ax} < 1; \Delta_r > 0$. 

\hspace*{\algorithmicindent} \textbf{Parameter units: } The units of  $\Delta_r$ is length; the units of $\beta$ is inverse length,  all the other parameters are dimensionless\\
\begin{algorithmic}[1]
\STATE Estimate/take as a reasonable constant $R_{cut}^{outer}$
\STATE $R_{cut}^{outer} \gets R_{cut}^{outer}(1 + \gamma)$
\FOR {$i, j: r_i, r_j \leq R_{cut}^{outer}$}
  \STATE $psm_{ij} \gets \text{SmoothMax}_{\beta}(\{r_i, r_j\}) + T(\beta)$
  \STATE $p_{ij} \gets f_c(r_i | R_{cut}^{outer}, C) f_c(r_j | R_{cut}^{outer}, C) q(\lVert \hat{r_i} \times \hat{r_j}\rVert_2^2 | \Delta_{ax}, C)$
\ENDFOR
\STATE $R_{cut}^{inner} \gets {\text{SmoothMinWeighted}_{\beta}}(\{(psm_{ij}, p_{ij})| i, j: r_i, r_j \leq R_{cut}^{outer}\} \cup \{(R_{cut}, 1.0)\})$
\STATE $R_{cut}^{inner} \gets R_{cut}^{inner} (1 + \gamma)$
\STATE $qsm \gets \underset{i, j: r_i, r_j \leq R_{cut}^{inner}}{\text{SoftMaxWeighted}_{\beta}}({\lVert \hat{r_i} \times \hat{r_j} \rVert}_2^2, f_c(r_i | R_{cut}^{inner}, C) f_c(r_j | R_{cut}^{inner}, C))$
\STATE $w_{ax} \gets q(2\Delta_{ax} -  qsm| \Delta_{ax}, C) $
\FOR {$i, j: r_i, r_j \leq R_{cut}^{inner} $ \textbf{ and } $i < j$}
\STATE $w_{ij} \gets fc(r_i | R_{cut}, C) fc(r_j | R_{cut}, C) q({\lVert \hat{r_i} \times \hat{r_j} \rVert}_2^2 | \Delta, C)$

\IF{$w_{ij} > 0$}
\SWITCH{$r_i - r_j$}
    \CASE{$r_i - r_j \geq \Delta_r$}
      \STATE $\text{Prediction}_{ij} \gets IM(D_{X} [g^{-1}_{ij}]\chi)$
    \ENDCASE
    \CASE{$-\Delta_r < r_i - r_j  < \Delta_r$}
      \STATE $\text{Prediction}_{ij} \gets \frac{
 IM(D_{X} [g^{-1}_{ij}]\chi) q(r_i - r_j | -\Delta_r, C) + IM(D_{X} [g^{-1}_{ji}]\chi) q (-(r_j - r_i) | \Delta_r, C)}{q(r_i - r_j | -\Delta_r, C) + q (-(r_j - r_i) | \Delta_r, C)}$
    \ENDCASE
    \CASE{$r_i - r_j \leq -\Delta_r$}
      \STATE $\text{Prediction}_{ij} \gets 
 IM(D_{X} [g^{-1}_{ji}]\chi)$ 
    \ENDCASE
\ENDSWITCH
\ENDIF
\ENDFOR
\IF{$w_{ax} > 0$}
    \STATE $\text{Prediction}_{ax} \gets AM(\{\vec{r_k}\})$
\ENDIF
\STATE $\text{Prediction} \gets \frac{\text{Prediction}_{ax}  w_{ax} + \sum\limits_{i > j: r_i, r_j \leq R_{cut}^{inner}} w_{ij} Prediction_{ij}}{w_{ax} + \sum\limits_{i > j: r_i, r_j \leq R_{cut}^{inner}} w_{ij} }$
\end{algorithmic}
\end{algorithm}
\twocolumngrid
\section{Fitting scheme}

There are two possible approaches to fit the model with symmetrization protocol. The first one immediately constructs rotationally invariant functional form and fits it as a whole. This way, though, is not very computationally efficient since initial model is invoked several times for the same configuration for every pass during the fitting process. An alternative approach is to fit initial model separately, and turn on symmetrization protocol only for subsequent atomistic simulations. In this case it is beneficial to use rotational and/or inverisonal augmentations to increase the generalization ability of the initial model. Since the functional form of symmetrization protocol is a weighted average of the predictions of initial model for several rotations the accuracy of symmetrization protocol is expected to be somewhere in between the accuracy of single evaluation of initial model and fully converged test rotational augmentations. This observation highlights that the several runs of the initial model implied by symmetrization protocol can be seen as not only the price to enforce exact rotational equivariance, but also as the rotational augmentations during testing which most of the time improves the accuracy. For the forces situation is not so straightforward since weights and reference frames in SP themselves depend on the positions of the atoms. Thus, when the initial model is fit, the fine-tuning of overall functional form might be required. In our experiment, though, for the dataset of randomly displaced methane configurations[] that we discuss in supplementary, we observe that the accuracy in forces for symmetrization protocol matches the one of initial model, even is slightly better, even without the fine-tuning. \mycomment{discuss potential reasons that the model is super rotationally invariant?}


* additional test augmentation if necessary
\begin{widetext}
    \begin{equation}
SP(\chi) = \frac{\sum\limits_{i, j} w_{ij} \frac{1}{N_{aug}} \sum\limits_{s}^{N_{aug}} D_{Y}[g_{ij}] D_{Y}[g_{aug}] IM(D_{X}[g^{-1}_{aug}]D_{X} [g^{-1}_{ij}]\chi) }{\sum\limits_{ij} w_{ij}}
\end{equation}
\end{widetext}


\section{Miscellaneous}
The presented symmetrization protocol defines a globally smooth approximation of the target property for all the positions except the ones where points collide with each other. The assumption of non-colliding points is not restrictive since, for such cases, corresponding nuclear reactions can not be described within the Born–Oppenheimer approximation, and thus, the very description of an atomic system as a point cloud becomes meaningless. 


\mycomment{
The approach used in the first version of DeepMD, where a single reference frame is defined by the closest pair of neighbors, can be seen as an instantiation of the FA framework alternative to what FA suggests for rotational equivariance itself. While one can say that the same applies to symmetrization protocol in spirit, formally, it can not be cast to the FA framework because of the usage of weighted averaging.}


On top of/instead symmetrization protocol one can handle the inversion group as:
\begin{equation}
SPI(\{r_k\}_k) = \frac{SP(\{r_k\}_k) + \alpha SP(\{-r_k\}_k)}{2}\text{,}
\end{equation}
where SPI = Symmetrization Protocol Inversion. $\alpha = 1$ for true scalars, and $\alpha = -1$ for pseudoscalars. The same scheme can be applied also to the rotationally covariant properties, for instance, to predict true and pseudo vectors. 


covariant predictions by "scalars are universal"





\clearpage
\section{not forget to insert somewhere}
* Improved description of atomic environments using low-cost polynomial functions with compact support. M discusses a lot of cutoff funcitons $f_c$, worth to discuss and cite.

* adaptive outer cutoff

\section{probably not to insert}

\begin{figure}[tb]
    \centering
    \includegraphics[width=0.8\linewidth]{figures/message_passing_scheme.png}
    \caption{message passing scheme}
    \label{fig:message_passing_scheme}
\end{figure}


Fig. \ref{fig:example_plane}
\begin{figure}[tb]
    \centering
    \includegraphics[width=0.8\linewidth]{figures/example_plane.jpg}
    \caption{example plane}
    \label{fig:example_plane}
\end{figure}

* [probably not] example how the covariant vector, aka dipole moment is automatically enforced to be within the plane if configuration is 2D. 
$\hat{R}_{ij}[\{\vec{r_k}\}])] = $
\begin{equation}
a
\end{equation}


\newpage

\fulfilled{these points are discussed in the text}
\newline
\notfulfilled{these points are not discussed in the text}
\newline
these points are unclassified yet
\newline

\notfulfilled{about utility function $q$: In addition, it is possible to show that if $w$ is treated as a variable instead of a parameter, the corresponding 2-dimensional function $q(z, w |C)$ is infinitely many times continuously differentiable in the domain defined by $w > 0$. }

\notfulfilled{[optional] discuss the difference between a priori and a posteriori symmetrization by mentioning the integral over rotations definiton of the invariants discussed above, and mentioning that it is not possible to integrate analytically arbitrary complicated neural network. }



* discuss simpler approach with auxiliary model. Discuss that this is a super rare case, both in the benchmark datasets and real life, and that this is never happening for 2d and 3d crystals, so the quality of the auxiliary model has a secondary importance. Mention that AX is turned on only in the nearest proximity of all collinear singularity, thus, has a small influence on the overall accuracy, and can be chosen as any model developed for atomistic machine learning internally covariant/invariant.  







* discuss more complicated approach which doesn't require an auxiliary model. Discuss continuous, refere differentiability to SI (if it has this property). 




So it is defined everywhere except the exact singularity of an exactly linear molecule. In the proximity of the singularity, reference frames are not stable, and rotate like crazy, but they do not have any impact on the prediction, and it converges to the expression illustrated in Fig. (). We provide more details in the SI.

* problem with collinear triplets and solution

* problem with $r_cut$ and solution [make sure that it is discussed before that global smooth approximation requires smoothness with appearence of the new atoms on the cutoff sphere if we use atomic decomposition of the target property]




[optionally] discuss deep md initial scheme and stress that while it is easy to obtain the symmetries separately (example with their rotationally invariant model with smoothness sacrifaction) it is a challenge to get all the symmetries simultaneously. And our protocol solves this. 

[discuss somewhere in the introduction the overall structure of symmetrization protocol that it involes evaluation of the model within several reference frames]

Symmetrization protocol: (model, point of interest) $\rightarrow$  global approximation of the target property with all the symmetries. 

* idea with a single reference frame which doesn't work "To the best knowledge of the authors there is no scheme designed which defines a single reference scheme in a smooth way, which is probably not possible because of the presence of highly symmetric configurations"

* Core idea with the all reference frames

$\hat{R}$ means only rotation because the defined reference frame is always right handed and, thus, inversion is not required. 





* problem with all-collinear configurations. discuss that there are two approaches to solve this. The first one which do not require auxiliary model but not able to work with covariant properties (as will be discussed later) and the one which does, but is able to predict covariant targets. 




locality of quantum mechanics, energy is extensive property, so it is typically decomposed into the sum of atomic contributions which depend on the local environments with in some cutoff radius. For the intensive properties, such as ..., one can use mean pooling instead of summation one. Such atomic environments are described by invariant features ... 

\subsection{models themselves}
models based on invariant features - BP neural networks based on symmetry functions; powerspectrum as the same thing. Higher order features ace, and the corresponding BP like functional form. 



Covariant features are not invariant ones, but the ones which transform in a predictable manner under rotations. Example is vector, tensor. Second example is l vector. Clebsch-Gordan iteration here. (provide also a "classical" name for this, which is probably tensor product). Cite here clebsch-gordan nets, nice (anything else?) 

Message passing is added to both approaches. ([based on invariant internal coordinates, 2-body distances schent, 3-body angles dimenet, 4-body gemnet ...]schnetpack, gemnet, and 3-body from new postdoc) (cormorant, nequip, tensor field network, mace)

Transformer can be done, where attention coefficients are invariants, tokens are covariant, thus, output is also covariant. 

\notfulfilled{
* discuss that while in principle such architecture can be made approximately rotationally invariant by rotational augmentations, and while in principle in some cases one can obtain something useful in some atomistic simulations, it adds one another headache to analyze the effect of not exact invariance and/or smoothness. Because of this "to the best of authors' knowledge None of the architectures described in previous section were ever applied to atomistic simulations, and so, the development in this and atomistic communities is isolated from each other"}


The intuition behind our model is very straigtforward. This model operates with a sequence of input tokens, and is intrinsically permutationally covariant (thus, when this property is undesirable positional encoding is added additiionally). This is an excellent match with the symmetry requirement for the model being permutationally invariant with respect to different enumerations of the atoms. As it was discussed in the section \ref{sec:atomistic_models} due to locality of quantum mechanics and the fact that the energy [make sure that I mention before that out of all the targets energy is the most prevalent one] is extensive property it is modelled as the sum of atomic contributions depending on the corresponding atomic neighborhoods. The very fundamental description of an atomic environment is given by the set of displacement vectors from central atom to all the neighbors along with information about the corresponding atomic specie. Thus, it is very natural to feed this very raw representation into a permutationally covariant model, such as Transformer or deep set to construct fully end-to-end permutationally invariant model. The overall scheme is illustrated in the Fig. {}. [discuss all the symmetries here], while the rotational symmetry is achieved by applying symmetrization protocol on top of this construction. 

\fulfilled{discussion of the modification of attention mechanism to ensure smoothness with respect to appearence of new atoms at the cutoff sphere. }

\section{was in symmetrization protocol session}


The parameter $\beta$ plays an important role in the \textit{SoftMax} function. If it is selected to be small the resulting approximation to the maximum is very smooth, but at the same time deviations from the exact maximum are large. On the contrary, for the large $\beta$ \textit{SoftMax} approximation is very close the exact maximum, but it lacks smoothness becoming more and more sharp. In the limit of infinite $\beta$ \textit{SoftMax} approximation converges to the exact maximum and becomes not differentiable. 

Our computational scheme for estimation of an adaptive cutoff exhibits the same behaviour ... "collectivelly refer to as $\lambda$" if they are selected to be tight, than ... , if loose, than ... . In the limit it converges to initial not working scheme by deepmd (a bit different due to filtering collinearity) the cusp is given as $\frac{rotational invariance}{size of transition region}$ thus the more rotationally invariant is the model out of the box the more tight $\gamma$ can be selected, and thus, the more efficient is the protocol. 



*[add a section(paragraph) (think where?) that there is additionally full control over the inversion symmetry, and mention it immediatelly during the first description of what the symmetrization protocol does]


* computational efficiency - discuss that currently it is a catostrophy, but can be done efficient

* simple solution with two different cutoffs, one for the model, second for the reference frames

* adaptive cutoff with all softmin machinery


* [think more] unite all the things together, such as to make sure that inside inner cutoff there is non collinear reference frame, not just any [may be put this into the SI]

* summary with mentioning that the full rigorous description of the protocols (both versions) is in the SI along with the proof of smoothness (while all the other properties are obvious)

* mention that this protocol also works for the current approaches of long-range interactions - both for behler charges, which are invariant functions of local atomic environments, and lode, where local object is designed to encapsulate long range information


\section{role of softmin parameters and fitting scheme}
*  two fitting schemes, of whole symmetrization protocol and rotational augmentations with only applying symmetrization protocol in the end. The second is more computationally efficient, since one need to compute several base models only during test, not during the train, so in the current work we use only it. It is not necessary to turn on train augmentation for the invariance properties of the final predictions, only for generalization.  [explore the other one as the future work]. Mention that one can also add also inversional augmentation depending if the target is inversionally invariant, though in our experiments this improves the test accuracy just a bit compared to the massive improvement from rotational augmentation. 

* mention that augmentations during the train are optional, only to increase generalization ability, SP produces exactly rotationally invariant and smooth model for any, even not fitted at all, IM  ("We stress that ")

* potential requirement for additional tuning on forces [mention that in our experiments model is out of the box so good that this is not required]

*  mention that one can see this not as a pure waste of resource but the test augmentation which also might be beneficial [find ref somewhere for this?]

* The mentioned above parameters of symmetrization protocol itself determine computational efficiency, for the proper selection, there is just one evaluation of the base model in general parameters, but there is some tradeoff, and it should be discussed in more details:

* [discuss the role of parameters used in the softmin, that smaller (may be bigger) they are the smaller are the margins upon the closest reference frames, and, thus,  for sufficiently large/small parameters in the general position only one reference frame is used. At some moments there would be transition from one reference frame to another and parameters determine the width of these transition. So there is a tradeoff between the computational efficiency and the amplitude of the spurious forces. The more rotationally invariant is the model out of the box, the smaller the softmin parameters can be selected, and thus, the more efficient is the general scheme. ] $\leftarrow$ think more about this

* discuss strategy to enforce additional rotational invariance [read before writing this about distillation] Discuss potential sampling in the domain of interest, aka molecular dynamics. Since contemporary neural networks have very huge number of parameters, and typically fit train data almost perfectly this is very promising strategy to determine additional computational efficiency. 

\section{application to atomistic machine learning}
* Symmetrization protocol requires not only the base model. There is a perfect match with locality of quantum mechanics and corresponding decomposition of the energy into the sum of atomic contributions. This includes the message passing schemes, as they also could be casted into atomic contributions paradigm. There is, though, additional computational cost, that message passing should be performed several times instead of ones. [probably do a picture to explain this]. 

* An alternative approach is to apply symmetrization protocol for each node independently, but in this case we need to enforce messages to invariant, and not the covariant ones. 

* for covariant messages train augmentation should be the global rotation of the whole system, and so the model is able to learn covariant messages. for invariant one we need to do independent local augmentations for all atomic environments, and thus, the model has no choice but learn invariant messages. 

* [covariant messages are more beneficial, since the feasibility of the model to communicate covariant inform  ation increase an expressive power. As will be shown later, our experiments demonstrate very consistently that covariant messages are more bene] $\leftarrow$ probably not

* Thus, this is very general and all the methods discussed in sec. \ref{sec:general_architectures} can be applied for atomistic machine learning using this protocol. [discuss maybe in more details]

* The is a great room to improve computational efficiency of a general symmetrization protocol in some particular cases. In some circumstances, it is possible to enable covariant messages without additional computational cost. For finite systems, such as molecules and small nano particles, we can select the single point for symmetrization protocol as center of the mass. While from mathematical point of view this is a working strategy for systems of any size, practically for too big systems point just around the center of the mass would have too big influence on the total energy since they determine the reference frames. [other example is global pool of reference frames for periodic systems with pruning by atomic species]


\section{in discussion}
Reasons to go for non equivariant with this symmetric protocol
[think more] other datasets, not from atomistic machine learning that people do not use not invariant models even when the target is invariant. 


[repeat some arguments from scn, and from force net if it has any] flexibility and blah blah blah. 

practical demonstration
PET, force net, SCN. 

discuss the situation from the point of view of completeness "for equivariant model it is a challenge to construct complete model, while for general one it is a challenge to construct not complete one"

* Mention that while for current methods with feature engineering every small step took separate development, aka separate article, and in general it took almost a decade to do all the things such as covariant input and output, here everything is out of the box [think more, probably softed the formulation] 


\subsection{discussion of the properties of our model and comparison with the others}
* single layer of this GNN is complete because transfomer can learn the same as deep set, and deep set is complete
* transformer itself is a gnn, so this is gnn embedded in gnn, "localised message passing", which is super beneficial since complex transformation might be introduced without the increase of the receptive field too much. Same trend with allegro and mace that single layer is strong, but the total number of layers is small.

\section{Introduction}
point clouds arise in various domains
examples, among the others, are rgb-d cameras and lidar. One another important example is atomistic machine learning. This case is unique because of additional complexity is the necessity to full-fill certain symmetries. [describe here two examples from the presentation for rotational invariance and smoothness]. 



Most of the methods developed for other cases do not full fill this requirements out of the box, and thus, are not applicable for atomistic machine learning. Because of this, despite the fundamental similarity of the structure of the data communities working on atomistic machine learning and the other 3D point clouds are completelly isolated from each other \{rephrase so it is not exactly the same sentence as in abstract\}. Out of the 4 mentioned required symmetries, though,  the only really problematic one is rotational invariance. As we discuss later most of the methods designed for generic point clouds already fulfill permutational and translational invariance, while ensuring smoothness is typically as trivial as changing the activation from ReLU to the smooth one. Our main contribution is general a posteriori rotational symmetrization protocol which takes arbitrary globally smooth, but not necessarily rotationally invariant, model, and produces simultaneously globally smooth and rotationaly invariant approximation of the target property suitable for atomistic simulations. 


This eliminates the wall between communities making most of  the models developed for general 3D point clouds suitable for atomistic simulations. The lack of necessity to explicitly incorporate rotational invariance into the functional form of the model allows not only to conduct atomistic simulations with the models previously developed for generic point clouds but also expands the horizons in developing the new, potentially more efficient architectures. We demonstrate this by achieving state of the art on a randomly displaced methane configurations, hme21 and coll datasets with the model we call Point Edge Transformer (PET) which becomes applicable for atomistic simulations if using presented symmetrization protocol. The paper is structured as follows - section \ref{sec:atomistic_models} contains brief discussion of methods designed for atomistic machine learning which explicitly incorporate rotational invariance; section \ref{sec:general_architectures} discusses architectures developed for general point clouds and required modifications make them smooth; section \ref{sec:symmetrization_protocol} contains symmetrization procol; section \ref{sec:PET} contains description of PET; section \ref{sec:state_of_the_art} contains state of the art achieved by PET and finally section \ref{sec:simulations} demonstrates applicability of PET for atomistic machine learning [I want to compute something simple like vibrational spectra there]
[While in principle it might be possible to get some meaningfull results from atomistic simulation with not exactly rotationally invariant model, it is not the case for majority of simulations, and it adds additional complexity of analyzing the potential artefacts caused by the lack of symmetries in the force-field. As a consequence such simulations are extremely rare, and typically force-fields used are not the ones from the other subfields of point clouds, but something new developed]


\section{old abstracts}
Processing point clouds in 3D space is an increasingly more important subfield of geometric deep learning. Atomistic configurations are an example of such objects, where points represent the positions of atomic nuclei. Other examples include the data from lidars, RGB-D cameras, and many others. Despite the fundamental similarity of the structure of the data, communities working on atomistic machine learning and the other 3D point clouds are completely isolated from each other. The reason for this are additional symmetry requirements for the models to be suitable for atomistic simulations, with the most challenging one of the model being \textbf{exactly} rotationally invariant. We eliminate this wall between the communities by designing a computationally efficient a posteriori symmetrization protocol making most of the models for point clouds applicable to atomistic simulations. We prove the usefulness of this approach by achieving state-of-the-art results on hme21, coll(?), randomly displaced methane configurations, and several other datasets with the model we name Cartesian Transformer with Message Passing (CTMP). In addition, we practically demonstrate the applicability of such established models as pointnet++ and [smth with voxels probably] to atomistic modeling if using our protocol by computing [vibrational frequencies ???] with these models. 

\mc{
Point clouds provide a very versatile description of three-dimensional shapes, and are used extensively in geometric deep learning, with applications ranging from autonomous driving and facial tracking to chemical and materials modeling. 
Despite the common geometric structure, various application domains have developed mostly independently, with little cross-contamination and different requirements for the model structure.
For example, atomistic machine learning gives much emphasis to \emph{exact} consistency with rotational symmetry, which is not only desirable to improve data efficiency, but also necessary to avoid introducing artefacts in simulations. 
Frameworks that are used for generic 3D shapes do not usually enforce these requirements, which has hindered their application to chemistry. 
In this work, we present a simple and general strategy to rigorously include rotational symmetry into any permutation-invariant point-cloud model, eliminating this barrier to the translation of deep learning frameworks between different domains. 
We demonstrate the idea by applying established models such as pointnet++ and [smth with voxels probably] to atomistic modeling, and develop a model, that we name Cartesian Transformer with Message Passing (CTMP), that achieves state-of-the-art results on hme21, coll(?), randomly displaced methane configurations, and several other benchmark datasets.
MAKE A NOTE ON HOW THIS IS MADE POSSIBLE BY RELAXING THE REQUIREMENT ON EQUIVARIANCE
}


\begin{figure}[tb]
    \centering
    \includegraphics[width=\linewidth]{figures/symmetrization_protocol_summary.png}
    \caption{symmetrization protocol summary}
    \label{fig:protocol_summary}
\end{figure}


 \mc{GOT HERE}




We have developed a general symmetrization protocol, which takes arbitrary smooth, permutationally, and translationally, but not necessarily rotationally invariant model and produces an exactly rotationally invariant approximation for the target property keeping all the other properties. The most obvious benefit of our construction is the possibility to use most of the developments done for generic point clouds in atomistic simulations in the form of entire models or, at least, core building blocks. Apart from that, it simplifies the development of new, better architectures, from the point of view of various criteria, such as generalization ability, or the computational cost, by eliminating the necessity to explicitly incorporate the rotational invariance into the functional form of the model. 
One of the manifestations of this burden is that the huge ratio of the models developed for atomistic modelling appeared not to be universal approximators, whereas the majority of non-rotationally invariant models for generic point clouds are. 
There is fact evidence suggesting that, unless exact rotational equivariance is necessary, including it approximately through  augmentation might be the most effective strategy. 
%The foremost argument that fitting the model with augmentations is likely the more beneficial strategy compared to explicit incorporation of the required symmetries into the functional form is that when the latter is not absolutely necessary, the best results are achieved with the first approach. 
For instance, for the classification of 3D shapes presented in the modelnet40[] dataset, people typically use rotational augmentation around the vertical axis. Indeed, the plane doesn't turn into the piano, just being viewed from a different angle. Even though the target is invariant with respect to rotations at least around the vertical axis, the current state-of-the-art [] and most of the other models do not incorporate either full rotational invariance or only around the vertical axis into their functional form. 

For the domain of atomistic systems, we prove the same with our model called Point Edge Transformer \mycomment{by achieving state of the art in various domains ... discuss achievements and model here}
Independently, the same observation was done by ForceNet[] and Spherical Channel Network (SCN). The first one indicates that if one does not explicitly impose rotational invariance, it leads to a better tradeoff between the model expressiveness and computational cost and achieves it on the Open Catalysis dataset. 
The second one, while not being rotationally equivariant, achieves the current state-of-the-art on the same dataset. \mycomment{[check smoothness and other properties]} 
If using our symmetrization protocol, both models can be used for atomistic simulations without any artifacts related to the lack of rotational equivariance. 

%The usage of all the reference frames is the very demonstrative starting point to illustrate our approach, but, as it will be shown later, practically, our computation scheme is very much different from that using only a few, potentially only one in some cases, the reference frame for each atomic environment most of the time, which makes it computationally efficient. 




%It is a complicated question if an approximate invariance achieved by the usage of rotational augmentations during the fitting is sufficient to conduct meaningful atomistic simulations. Probably there are some applications where it is possible to get reasonable results even with such a model. Though, 
\section{Symmetrization protocol shortened}




\section{Symmetrization protocol}

Our construction accepts smooth, permutationally, translationally, but not necessarily rotationally equivariant model along with the point of interest and produces the functional form satisfying all four necessary requirements. While in principle, there are many choices of the point of interest, we will stick, for simplicity, to the local energy decomposition of equation \ref{eq:atomic_energy_decomposition} where the point of interest is given as the position of the central atom, and the model produces atomic energy $E_i$ given the local neighborhood of an atom $i$.

Each neighbor in an atomic environment is described by a displacement vector $\br_i$, label with atomic specie $s_i$, and potentially by some other, maybe equivariant, attributes. An example of these additional attributes are spins [discuss what are the spins, mention that spins can be scalar, vectorial and even higher tensro (ralf talks about vectorial spins)]. Finally, if the symmetrization protocol is applied within an equivariant graph neural network, additional covariant attributes of each neighbor are given by equivariant input messages from the previous layer. Application of SP to message passing scheme is described in more detail in sec. []. Collectivelly we refer to an atomic environment as to $\chi = \{(\br_i, s_i, ...)\}_{i = 1}^{N}$. 

A definition of a rotationally equivariant function $f: X \rightarrow Y$ is that it transforms in a certain manner with rotations:

\begin{equation}
    D_Y[g] f(x) = f (D_X[g] \chi) \quad \forall g \in SO(3), \forall \chi \in X\text{,}
\end{equation}
where $D_X[g]$ and $D_Y[g]$ denote representations of a rotation $g$ in vector spaces $X$ and $Y$. Examples of rotationally equivariant targets include vectorial dipole moments, tensorial polarizabilities. Also, 


\mycomment{[probably only in SI] discuss that symmetrization protocol requires two points should not collide, that it is a nuclear reaction, BO approximation and blah, blah, blah}
\label{sec:symmetrization_protocol}
\subsection{Preliminaries}
\begin{figure}[tb]
    \centering
    \includegraphics[width=0.8\linewidth]{figures/utility_functions.jpg}
    \caption{Infinitely differentiable utility functions $f_c$ and $q$ defined in the main text.}
    \label{fig:utility_functions}
\end{figure}



Symmetrization protocol relies on several mathematical constructions on top of the $f_c$ function discussed in the previous section. 

The counterpart function $q$, which smoothly zeroes out the domain $z <= \Delta$ is shown in fig. \ref{fig:utility_functions} (b) and can be defined as:
 \begin{equation}
 q(z | \Delta, C) = 
    \begin{cases}
        exp(\frac{-C}{z / \Delta - 1}),& \text{if } z \geq \Delta\\
    0,              & \text{otherwise}
    \end{cases}\text{,} 
\end{equation}


A smooth approximation for the \textit{max} function of any finite set of numbers  $\{x_i\}_i$ can be defined for $\beta > 0$ as:
\begin{equation}
\text{SmoothMax}(\{x_i\}_i | \beta) = \frac{\sum\limits_i exp(\beta x_i) x_i}{\sum\limits_i exp(\beta x_i)}\text{.}
\end{equation}
It is possible to show that it satisfies the following properties:
\begin{equation}
\label{eq:smooth_max_basic_properties}
\begin{split}
\lim_{\beta \to +\inf}  \text{SmoothMax}(\{x_i\}_i | \beta) = max(\{x_i\}_i) \\
\text{SmoothMax}(\{x_i\}_i | \beta) \leq max(\{x_i\}_i)
\end{split}
\end{equation}

Finally, given an ordered pair of noncollinear unit vectors $\hat{v_1}$ and $\hat{v_2}$ we define associated reference frame by computing $\vec{u_1} = \hat{v_1} \times \hat{v_2}$, $\hat{u_1} = \vec{u_1} / \lVert \vec{u_1} \rVert$ and $\hat{u_2} = \hat{v_1} \times \hat{1_2}$. The reference frame is given by the vectors $\hat{v_1}$, $\hat{u_1}$ and $\hat{u_2}$. This procedure generates only right-handed coordinate systems, and thus, the change to them is always given by some rotation, never requiring inversion. When we later refer to the reference system given by a central atom and two neighbors $i$ and $j$, we mean that the vectors $\hat{v_1}$ and $\hat{v_2}$ are the ones pointing from the central atom to neighbors $i$ and $j$ respectively. 

\subsection{Core idea}
\begin{figure}[tb]
    \centering
    \includegraphics[width=0.8\linewidth]{figures/symmetrization_figure.pdf}
    \caption{(a) Discontinuities related to (dis) appearance of the new neighbor at the cutoff sphere and to an impossibility of defining a reference frame for a collinear triplet of points. (b)  all-collinear problem. The degree of the problematic narrowness of the cone depends on the parameter $\Delta$. (c) For exact all-collinear singularity SP converges to the depicted value in the case of the first solution to the all-collinear problem. IM model is applied to configurations where atoms are aligned along the x-axis}
    \label{fig:symmetrization_protocol}
\end{figure}

It is a very tempting idea to define somehow a reference frame associated with an atomic environment. Indeed, in this case, one can just project all the displacement vectors from the central atom to all the neighbors to this reference frame and feed the result to any, not necessarily, rotationally invariant model. Since the reference frame rotates together with the atomic environment, the projections of all the displacement vectors are invariant with respect to rotations, and so is the final prediction of the model. The problem with this approach is, though, that it is not known how to define such a reference frame in a smooth manner. An example is the first version of DeePMD[], which uses a reference frame defined by the central atom and two closest neighbors. The problem with this approach is that if the closest pair switches, it leads to the discontinuous jump of the reference frame, and subsequently to the discontinuity in predictions.

Another example of ensuring rotational equivariance by sacrificing smoothness is given in FA framework\cite{puny2021frame}. Its instantiation for rotational equivariance suggests using eigenvectors of the covariance matrix to construct the reference frame. Since the eigenvectors are defined up to the sign, all possible $2^3$ collections of signs are used. As \cite{puny2021frame} itself indicates, eigenvectors of the covariance matrix are discontinuous in the degenerate configurations where two or more eigenvalues are the same.  

The core idea of our symmetrization protocol is extremely simple. One can use all the possible reference frames defined by the all pairs of neighbors instead of any single one and average predictions over all of them:


\begin{equation}
\label{eq:all_ref_frames_simplest}
    SP(\chi) = \frac{\sum\limits_{i, j} D_{Y}[g_{ij}] IM(D_{X} [g^{-1}_{ij}]\chi)}{N_{pairs}}
\end{equation}
Where $SP$ means Symmetrization Protocol, $IM$ means Initial Model, and $\hat{R}_{ij}(\cdot)$ denotes projection onto reference frame defined by central atom and neighbors $i$ and $j$, or, equivalently, the operator performing the corresponding rotation. 

The idea of using all the possible reference frames also constitutes the base of Weighted Matrices Invariant(WMI)[Vitaliy] and 3-centered SOAP introduced in []. The first one is focused on the crystal structure matching problem and applies it to define a polynomialy computable metric between the two crystals, which is zero if and only if two crystals are exactly the same with respect to rigid transformations. The second one defines complete descriptors suitable for atomistic machine learning for the environments of each triplet of the atoms in the system. 

The usage of all the reference frames is the very demonstrative starting point to illustrate our approach, but, as it will be shown later, practically, our computation scheme is very much different from that using only a few, potentially only one in some cases, the reference frame for each atomic environment most of the time, which makes it computationally efficient. 

The most straightforward formulation of Eq. \ref{eq:all_ref_frames_simplest} still contains a few sources of discontinuity to be eliminated. The first one is related to the (dis)appearance of a new atom on the cutoff sphere as illustrated in Fig. \ref{fig:symmetrization_protocol} (a). When this happens, the new atom immediately contributes new reference frames and, subsequently, new terms to the nominator of eq.  \ref{eq:all_ref_frames_simplest}, which instantly leads to the jump in the predictions. In order to fix this symmetrization protocol can be reformulated as:


\begin{equation}
\label{eq:weighted_average}
SP(\chi) = \frac{\sum\limits_{i, j} w_{ij} D_{Y}[g_{ij}] 
 IM(D_{X} [g^{-1}_{ij}]\chi) }{\sum\limits_{ij} w_{ij}}\text{,}
\end{equation}

where  $w_{ij} = fc(r_i | R_{cut}, C_{fc}) fc(r_j | R_{cut}, C_{fc})$. 

Now, when the new atom enters the cutoff sphere, the new terms associated with it have zero weight and, thus, do not affect discontinuously the result of the weighted average. 

The second problem is that it is impossible to define a reference frame for a pair of neighbors that form a collinear triplet with the central atom, as shown in Fig. \ref{fig:symmetrization_protocol} (a). One can tackle this issue similarly to the previous modification, smoothly zeroing out contributions from the pairs of neighbors that are close enough to be collinear. The weights in the weighted average \ref{eq:weighted_average} can be selected as:

\begin{equation}
\label{eq:weight_full}
w_{ij} = fc(r_i | R_{cut}, C_{fc}) fc(r_j | R_{cut}, C_{fc}) q({\lVert \hat{r_i} \times \hat{r_j} \rVert}_2^2 | \Delta, C_{q})\text{.}
\end{equation}

The non-dimensional squared norm of a cross product of unit vectors pointing to neighbors $i$ and $j$ plays the role of numerical degree of collinearity, and constant parameter $\Delta > 0$ controls the boundary determining which reference frames are considered to be stable enough to be used in symmetrization protocol, and which are not. 

The last and most complicated problem arises when it is impossible to define any stable reference frame, which is illustrated in Fig. \ref{fig:symmetrization_protocol} (b). For such a case of a narrow cone (the degree of problematic narrowness is determined by the parameter $\Delta$), all the weights defined in eq. \ref{eq:weight_full} are zeros, and the weighted average falls to the $\frac{0}{0}$ ambiguity.  We present two ways to fix this issue. The first one doesn't have any additional requirements but doesn't extend to the covariant inputs and outputs, only working with invariant ones,  which, though, is the prevalent case in atomistic machine learning. The second one requires an auxiliary internally invariant/covariant model, one of the ones discussed in sec. \ref{sec:atomistic_models} to handle narrow cone configurations. As it will be shown later, it is possible to extend this formulation of symmetrization protocol for covariant inputs and outputs. 

\subsection{First solution to the all-collinear problem}
The idea of the first approach is to make adaptive the parameter $\Delta$ that controls which reference frames are considered to be stable enough to be used in symmetrization protocol. Namely, one can put it as:
\begin{equation}
\Delta = 0.5 * \underset{ij}{\text{SmoothMax}}(\{{\lVert \hat{r_i} \times \hat{r_j} \rVert}_2^2\})\text{.}
\end{equation}

This makes the weighted average of symmetrization protocol to be well defined everywhere except the exact all-collinear singularity. Indeed, for arbitrarily narrow cone, we have that
\begin{equation}
\underset{ij}{\max}(\{{\lVert \hat{r_i} \times \hat{r_j} \rVert}_2^2\}) \geq \underset{ij}{\text{SmoothMax}}(\{{\lVert \hat{r_i} \times \hat{r_j} \rVert}_2^2\}) = 2\Delta \text{,}
\end{equation}
which at least leads to nonzero weight for the corresponding most noncollinear reference frame:

\begin{equation}
q(\underset{ij}{\max}(\{{\lVert \hat{r_i} \times \hat{r_j} \rVert}_2^2\}) | \Delta, C_{q}) \geq q(2 \Delta| \Delta, C_{q}) = exp(-C_{q})
\end{equation}

Though in the proximity of exact all-collinear singularity, the reference frames themselves used by symmetrization protocol are not stable, it is possible to show that the output of symmetrization protocol itself converges to the value we schematically illustrate in Fig. \ref{fig:symmetrization_protocol} (c). Thus, extending the definition of symmetrization protocol to the all-collinear configurations in such a way leads to a globally continuous approximation of the target property. 

\subsection{Second solution to the all-collinear problem}]
\mycomment{discuss that the case when the auxiliary model is used is very rare in real life}
The idea of the second approach is to apply an auxiliary model for the problematic narrow cone configurations and next smoothly stitch it with the main model, which handles all the others:

\begin{equation}
SP(\chi) = w_{ax} \frac{AM(\chi)  + \sum\limits_{i, j} w_{ij} D_{Y}[g_{ij}] 
 IM(D_{X} [g^{-1}_{ij}]\chi) }{w_{ax} + \sum\limits_{ij} w_{ij}}\text{,}
\end{equation}
where $AM$ denotes Auxiliary Model build to be internally invariant with respect to rotations, and the weight $w_{ax}$ is defined as:

\begin{equation}
w_{ax} = q(2\Delta_{ax} - \text{SoftMax}(\{{\lVert \br_{i} \times \br_{j} \rVert}_2^2\}_{ij}) | \Delta_{ax}, C_{ax}) \text{,}
\end{equation}
where $\Delta_{ax} > \Delta$. This helps to avoid previously mentioned $\frac{0}{0}$ ambiguity for the narrow cones since the well-defined prediction given by the auxiliary model is admixed to the weighted average. At the same time, the auxiliary model is turned off for most configurations, namely when $ \text{SoftMax}(\{{\lVert \br_{i} \times \br_{j} \rVert}_2^2\}_{ij}) \geq \Delta_{ax}$. 

Since this construction involves only infinitely differentiable utility functions, it lifts up all the smoothness of the $IM$ and $AM$ models. That is if these models are $k$ times continuously differentiable, so is the functional form defined by the symmetrization protocol. 

\subsection{Covariant inputs and outputs}
The presented symmetrization protocol can be generalized to the prediction of covariant properties of molecules and materials of any kind with minimal effort and without the necessity of any modifications to the initial model. This can be done by transforming the predictions produced by an initial model for each reference frame used by symmetrization protocol to the reference frame of interest, with respect to that one needs to compute covariant property:
\begin{equation}
\label{eq:covariant_output}
SP(\{\br_{k}\}) = \frac{\sum\limits_{i, j} T_{ij}[IM(\hat{R}_{ij}[\{\br_{k}\}])] w_{ij}}{\sum\limits_{ij} w_{ij}} \text{,}
\end{equation}
where the operator $T_{ij}$ denotes the transformation rule. For example, if one needs to predict vectorial properties, such as dipole moments, then the $T_{ij}$ is given by multiplication with a 3 x 3 change of coordinates matrix $u_{ij}$. For a tensor of rank $K$,  $T_{ij}$ is given as:
\begin{equation}
T_{ij}(p)_{\alpha_1'...\alpha_k'}= \sum\limits_{\alpha_1 ... \alpha_k} 
 p_{\alpha_1...\alpha_k}\prod\limits_{k=1}^{k=K}[u_{ij}]_{\alpha_k'\alpha_k} \text{,}\end{equation}
which allows to directly predict covariant tensors of any rank. It is possible, though, to design a more computationally efficient strategy by 
recasting the tensor into its irreducible spherical tensor representation. In this case, operator $T_{ij}$ is given by multiplication with Wigner D matrices. 
\mycomment{cite Symmetry-Adapted Machine-Learning for Tensorial Properties of Atomistic Systems, and probably link 36 from there}

In addition to the prediction of covariant properties, sometimes there is a need to process covariant inputs when each point is supplied with some covariant variable that transforms together with the system. Generalization of symmetrization protocol to this case is even simpler than to covariant properties. One just needs to set the operator $\hat{R}_{ij}$ to transform these variables accordingly in addition to displacement vectors from the central atom to all the neighbors. 

\subsection{Computational efficiency}
Described so far symmetrization protocol requires running the initial model $O(N^2)$ times, where $N$ is the number of atoms within an atomic environment. This makes it computationally prohibitable to use in practice. The simplest solution is to use two different cutoff spheres. The first one is for the model itself, and the second one, selected to be small enough, for the symmetrization protocol. While this is a big improvement over the initial computation scheme, it is possible to do much better than this defining an adaptive $R_{cut}$ for each atomic environment. As we discuss in Supplementary, one can extend the idea behind \textit{SmoothMax} function to design a smooth approximation for a second minimum which is always greater or equal than the exact value of a second minimum. Next, one can feed all the distances $\{\lVert \br_{k}\rVert_2^2\}$ to this smooth second minimum function getting the approximation for the smallest sufficient value of $R_{cut}$ for symmetrization protocol. More precisely, our construction takes into account the potential collinearity of the two closest neighbors and the central atom and selects such a cutoff that there is at least one "good" ($\lVert \hat{r_i} \times \hat{r_j} \rVert_2^2 > \Delta$) pair of neighbors inside the cutoff sphere given that there is at least one in the whole system. On top of that, we do the additional cutting by using only one reference frame for each unordered pair of neighbors instead of two. This is achieved by selecting the more distant neighbor from the central atom to be the first one. In a small transition region, where the distances to both neighbors are close to each other, we use smooth stitching, similar in spirit to the one we applied for the second solution to the all-collinear problem. The same way as the smooth maximum converges to the exact maximum for sufficiently large $\beta$, our adaptive $R_{cut}$ becomes closer and closer to the minimal sufficient value the tighter the parameters analogous to $\beta$ in smooth max are. Thus, for sufficiently tight selection, in general position, only one reference frame is active most of the time.

\mc{
\subsection{Message passing}
MUST EXPLAIN IN THE MAIN. GENERAL CASE: VERY EXPENSIVE  
}

\section{Point Edge Transformer}

\label{sec:PET}

The most obvious benefit of the general symmetrization protocol is that it makes most of the developments for generic point clouds discussed in the sec \ref{sec:general_architectures} applicable for atomistic modelling. Benchmarking the great multitude of such models on atomistic datasets is, though, out of the scope of this paper. Instead, we focus on the second, less obvious, but not less pronounced, benefit that the burden of explicit incorporation of the rotational equivariance into the model is now eliminated, making the scope of potential functional forms in the neural network architectures much richer. It means that the search space of potential architectures is much bigger, making it easier to construct a better model from the point of view of various criterions such as generalization ability, computational efficiency, memory requirements, ability to capture certain chemical interactions, and so on. We demonstrate this with a model we name Point Edge Transformer (PET), achieving state-of-the-art in the various domains of atomistic machine learning.


The most fundamental description of an atomic environment is given by an unordered set of displacement vectors from the central atom to all the neighbors supplied with information about corresponding atomic specie. Transformers[], which produce a permutationally covariant transformation of the input sequence, are known to achieve excellent results in various domains ranging from natural language processing[] to computer vision[]. The permutationally invariant prediction can be achieved by the "cls" token strategy used by Bert[] and visual transformers[] to obtain the representation of the whole sentence or the whole image, respectively. This "cls" token is a very convenient place to put embedding of the specie (and other properties, if there are any) of the central atom. Thus, later we will call it a central token. On top of this, we construct a graph neural network where the permutationally covariant outputs of the transformer associated with each neighbor $j$ are treated as a messages from central atom $i$ to neighbor $j$. Computation of the new vertex features by typical GNN involves aggregation over all the neighbors. The proposed "aggregation-free" message passing avoids this step, and so the corresponding bottleneck of the information flow. All the mentioned considerations sum up to the architecture we illustrate in Fig. \ref{fig:architecture_PET}. 

\begin{figure*}[h]
    \centering
    \includegraphics[width=1\linewidth]{figures/architecture.png}
    \includegraphics[width=1\linewidth]{figures/architecture-scheme.pdf}
    \caption{architecture PET}
    \label{fig:architecture_PET}
\end{figure*}

The transformer encoder block is identical to the classical one from attention is all you need[] except the modification of the attention mechanism to ensure smoothness with respect to (dis)appearance of the atom at the cutoff sphere. The attention coefficients $\alpha_{ij}$ determining the contribution from token $j$ to token $i$ are modified as:

\begin{equation}
\alpha_{ij} \leftarrow  \alpha_{ij} f_c(r_j | R_{cut}) \text{,}
\end{equation}
with subsequent renormalization. 


There is great variability in the pre- and post-processing of tokens before and after feeding them to the transformer. \mycomment{Particularly [ discuss bonds, blending or not neighbors embedding, maybe linearities].} One possibility is especially peculiar, that is, if explicitly precompute or not the lengths of displacement vectors to each neighbor. Even though the length can be computed arbitrarily accurately by MLP1 and subsequently in the transformer, such preconditioning leads to a noticeable increase of model capacity and acceleration of the fitting process for the data-rich regime. This comes almost for free since the computational cost associated with explicit length computation is almost zero compared to the other parts of the model. For the data-poor regime, the effect of explicit length computation is not so unambiguous, sometimes leading to higher overfitting. 


The key difference of our model compared to other transformers developed for point clouds[] is that it assigns features to each edge within a certain cutoff radius in contrast to points as the other transformers do. The Edge Transformer[] does the same but is designed for NLP tasks \mycomment{and not for point clouds.}

There is a general trend outlined in sec. \ref{sec:atomistic_models} that GNNs developed for atomistic modelling perform increasingly more complicated operations in a single layer moving from two-body messages to three and even four-body. Interestingly, it also applies to rotationally equivariant architectures, such as Mace and allegro, even though nequip, as long as tft, are known to be universal approximators. 

Our model is in perfect agreement with this trend since each message-passing layer is given by an arbitrarily deep transformer, which is known to be a universal approximator[]. 

Since the transformer itself can be treated as a GNN[], our architecture can be seen as doing a localized message passing, avoiding an over-increase of the receptive field, which is believed to be one of the problems associated with deep GNNs[oversquashing link from Bernstein blog].

\mycomment{which is probably one of the reasons why deep GNNs are not that effective since it leads to over-squashing phenomena[]. }



\section{state of the art}
\label{sec:state_of_the_art}

\begin{table}
\label{table:coll}
\begin{tabular}{lS[table-format=3.1]@{\hspace{0.2cm}}S[table-format=3]}
& \mcc{Forces}              & \mcc{Energy}            \\
\hline
SchNet                & 172           & 198         \\
$\text{DimeNet}^{++}$ & 40            & 47      \\
GemNet-Q              &  26.4         & 53         \\
GemNet-T              & 31.6          & 60          \\
GemNet-dQ             & 38.1          & 60          \\
GemNet-dT             & 43.1          & 55          \\
PET                   & \bfseries \mycomment{23.85} & -     
\end{tabular}
\caption{coll results. The primary target for this dataset is the forces. Thus, the GemNet, which is a successor and improved version of DimenNet, has a higher error in energies. For simplicity, we use only forces.
\mc{ Running with energy targets. Expected energy error in the 20-30. ETA 1 week at worst. }
}
\end{table}

\begin{figure}[tb]
    \centering
    \includegraphics[width=\linewidth]{figures/sota_template.pdf}
    \caption{lc rmse of methane in energies if fitted (a) only on energies (b) on energies and forces.
    (c) lc rmse of high entropy alloys in energies (d) lc rmse of high entropy alloys in forces, (c) and (d) fitted on both energies and forces
    \mc{1.5x better than REANN at 10k when learning with forces. Running on 30k and 100k. Results on small model: 1 week, might have to go to larger model, then much slower. 
    Energy-only are also great but need re-running. For after preprint. 
    }
    }
    \label{fig:sota}
\end{figure}

\begin{figure}[tb]
    \centering
    \includegraphics[width=1.0\linewidth]{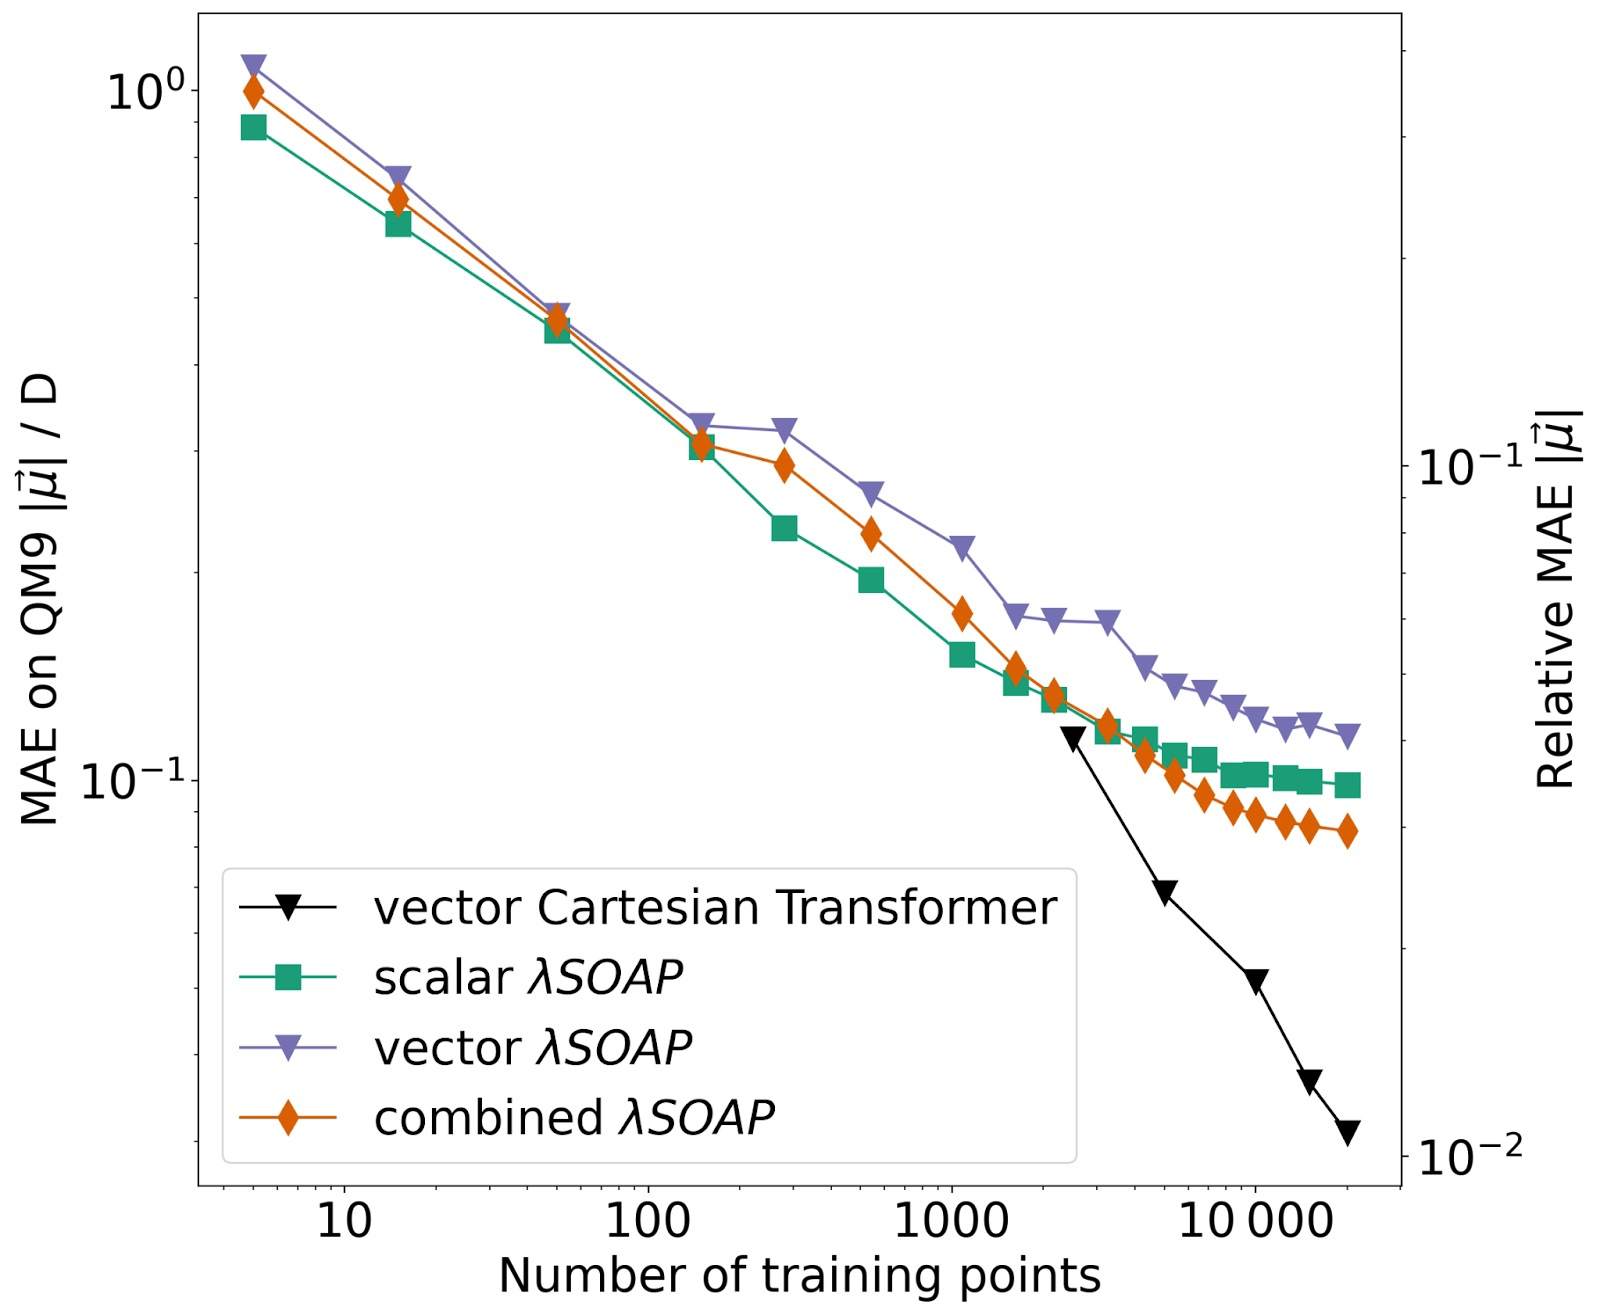}
    \caption{\mycomment{cut probably at least from about 300}}
    \label{fig:dipole}
\end{figure}



\begin{table}[hbp]
  \centering
  \begin{tabular}{lD{.}{.}{3}D{.}{.}{4}D{.}{.}{4}}
 & {Energy MAE} & {Force MAE}  & {Force XYZ MAE} \\
Architecture & {[meV/atom]} & {[eV/\AA]}  & {[eV/\AA]} \\ \hline
TeaNet  & {19.6} & {0.174} & {0.153} \\
SchNet & 33.6 & 0.283 & 0.247 \\
PaiNN & 22.9 & 0.237 & 0.208 \\
NequIP ($l_\mathrm{max}=0$) & 52.2 & 0.249 & 0.225 \\
NequIP ($l_\mathrm{max}=1$) & 53.3 & 0.233 & 0.206 \\
NequIP ($l_\mathrm{max}=2$) & 47.8 & 0.199 & 0.175 \\
PET & \mycomment{$\approx$ 16}& & \mycomment{$\approx$ 0.130}\\
  \end{tabular}
  \caption{ 
HME21 dataset. \mc{We roughly match MACE. Perhaps possible to do better, either tweaking learning schedule or extending the model. We stick with what we have, and start a large model training for later. }
  }
  \label{table:hme21}
\end{table}


Table \ref{table:coll} \ref{table:hme21}
Fig. \ref{fig:sota}, fig. \ref{fig:dipole}

\emph{
Behler spins
Pet errors:
Energy rmse $\approx$ 0.011 eV/structure $\approx $ 0.173 meV/atom, force rmse $\approx$ 0.008 eV/A. 
Behler errors:
energy rmse: 1.11 meV/atom, force rmse  $0.066 eV / a_0 \approx 0.13 eV/A$ 
triple check
\mc{Ten times better. Make figure and be happy}
}

\emph{
Bingqing Water model. 
\mc{Results are much better that SOTA, the ablation study is not complete. ETC 3 days  }
}

\section{Discussion}
\label{sec:discussion}
We have developed a general symmetrization protocol, which takes arbitrary smooth, permutationally, and translationally, but not necessarily rotationally invariant model and produces an exactly rotationally invariant approximation for the target property keeping all the other properties. The most obvious benefit of our construction is the possibility to use most of the developments done for generic point clouds in atomistic simulations in the form of entire models or, at least, core building blocks. Apart from that, it simplifies the development of new, better architectures, from the point of view of various criteria, such as generalization ability, or the computational cost, by eliminating the necessity to explicitly incorporate the rotational invariance into the functional form of the model. 
One of the manifestations of this burden is that the huge ratio of the models developed for atomistic modelling appeared not to be universal approximators, whereas the majority of non-rotationally invariant models for generic point clouds are. 
There is fact evidence suggesting that, unless exact rotational equivariance is necessary, including it approximately through  augmentation might be the most effective strategy. 
%The foremost argument that fitting the model with augmentations is likely the more beneficial strategy compared to explicit incorporation of the required symmetries into the functional form is that when the latter is not absolutely necessary, the best results are achieved with the first approach. 
For instance, for the classification of 3D shapes presented in the modelnet40[] dataset, people typically use rotational augmentation around the vertical axis. Indeed, the plane doesn't turn into the piano, just being viewed from a different angle. Even though the target is invariant with respect to rotations at least around the vertical axis, the current state-of-the-art [] and most of the other models do not incorporate either full rotational invariance or only around the vertical axis into their functional form. 

For the domain of atomistic systems, we prove the same with our model called Point Edge Transformer \mycomment{by achieving state of the art in various domains ... discuss achievements and model here}
Independently, the same observation was done by ForceNet[] and Spherical Channel Network (SCN). The first one indicates that if one does not explicitly impose rotational invariance, it leads to a better tradeoff between the model expressiveness and computational cost and achieves it on the Open Catalysis dataset. 
The second one, while not being rotationally equivariant, achieves the current state-of-the-art on the same dataset. \mycomment{[check smoothness and other properties]} 
If using our symmetrization protocol, both models can be used for atomistic simulations without any artifacts related to the lack of rotational equivariance. 
